# Supplementary material for: Constructing networks by filtering correlation matrices: A null model approach
Source: arXiv:1903.10805 source file (2019-03-26)
Supplement: Supplementary file 1 [file si.pdf]

# Constructing networks by filtering correlation matrices: A null model approach

Sadamori Kojaku and Naoki Masuda

## I. PREDICTION OF COUNTRY-LEVEL PRODUCT EXPORTS WITH OTHER NULL MODELS

For the product space data, we examine the prediction performance of the Scola combined with other null models for correlation matrices and precision matrices. The joint distribution of the actual and predicted $\overline{R}$ values is shown in Fig. 1. For both time windows, the MSE values for all the cases are larger than that for the original Scola combined with the configuration model (Fig. 4 in the main text).

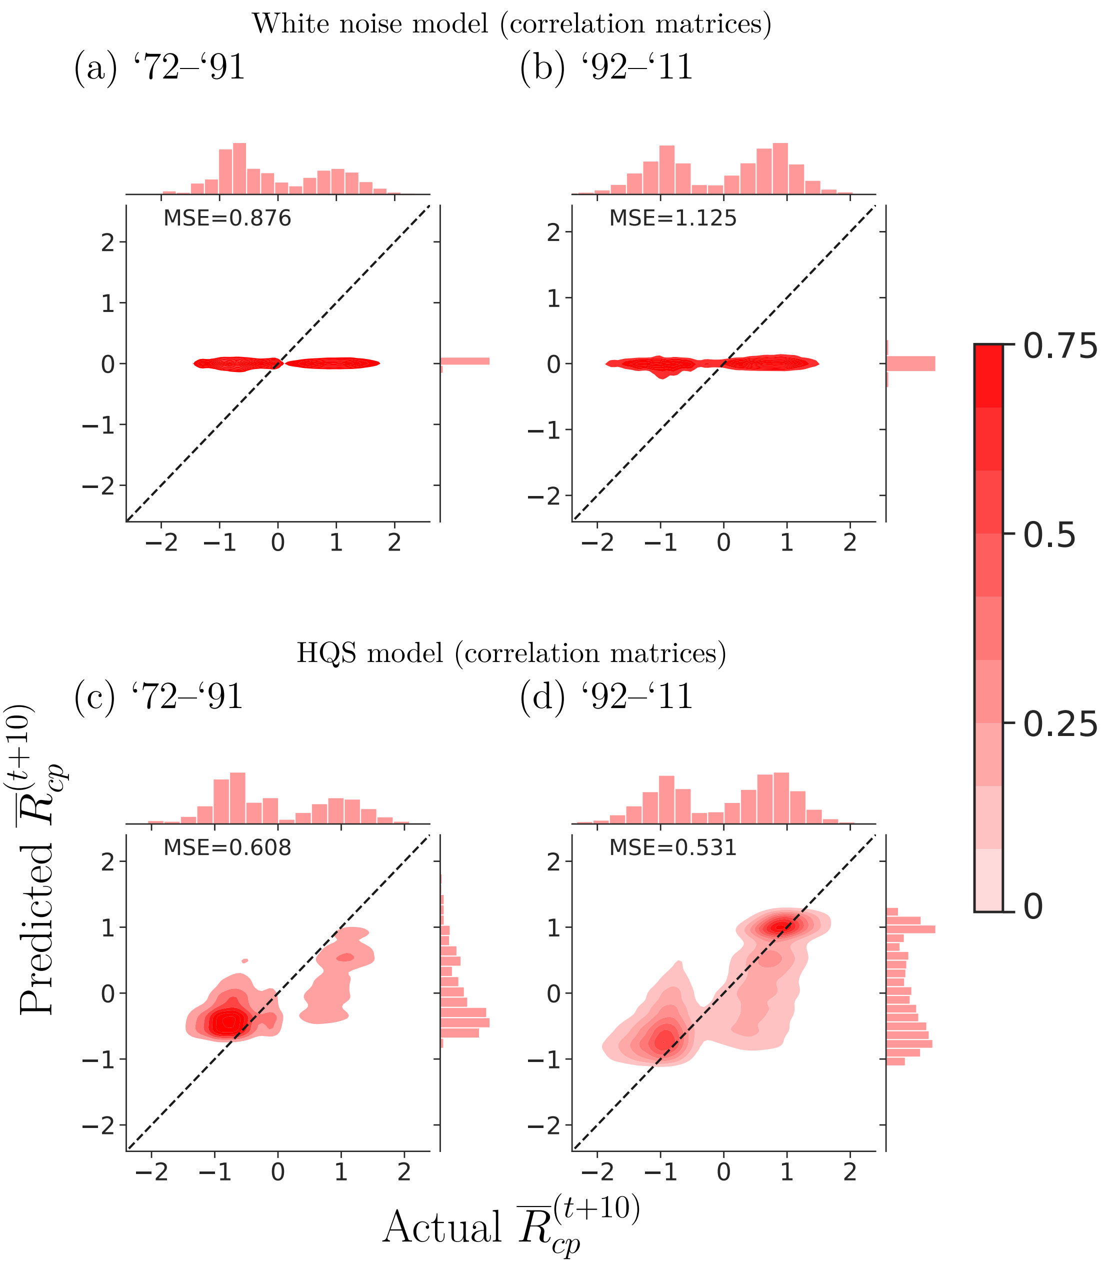


FIG. 1: Additional results on the prediction of product exports with the use of the Scola and its variant.

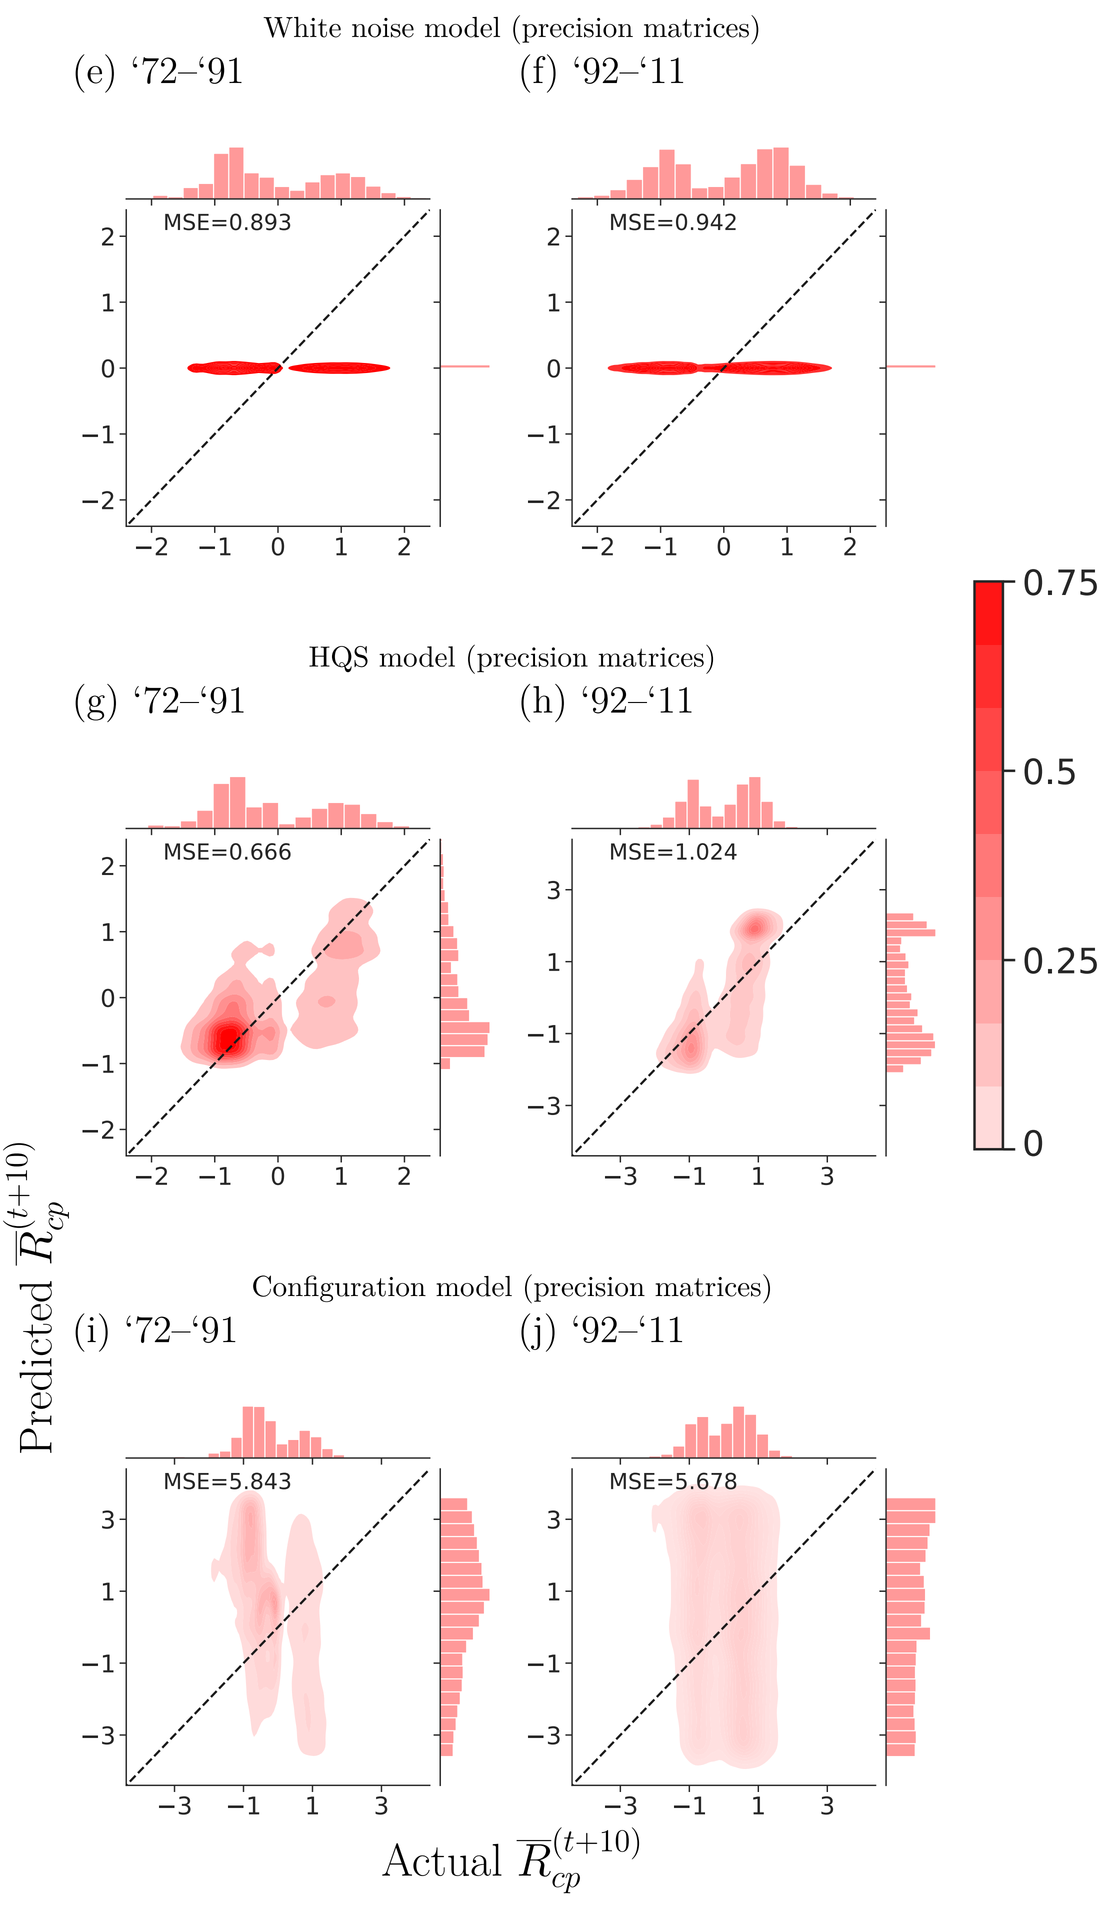
White noise model (precision matrices)
(e) ‘72–‘91
(f) ‘92–‘11
MSE=0.893
MSE=0.942
HQS model (precision matrices)
(g) ‘72–‘91
(h) ‘92–‘11
MSE=0.666
MSE=1.024
Configuration model (precision matrices)
(i) ‘72–‘91
(j) ‘92–‘11
MSE=5.843
MSE=5.678
Predicted $\overline{R}_{cp}^{(t+10)}$
Actual $\overline{R}_{cp}^{(t+10)}$
0.75
0.5
0.25
0
